# Supplementary material for: CoWeave: Identity-Specific Context Reasoning for Persistent Multi-Camera Tracking
Source: arXiv:2611.38993 source file (2026-11-28)
Supplement: Supplementary file 1 [file supp_coweave_style.tex]

\providecommand{\cwStyleLoaded}{}
\definecolor{cwA}{HTML}{5FB8C2}      % identity A, teal (fills, bars)
\definecolor{cwB}{HTML}{F2A0C8}      % identity B, rose (fills, bars)
\definecolor{cwC}{HTML}{B4A7D6}      % identity C
\definecolor{cwAd}{HTML}{1A7F8E}     % identity A, strokes and letters (4.6:1 on white)
\definecolor{cwBd}{HTML}{B8418A}     % identity B, strokes and letters (5.0:1 on white); magenta side, apart from the coral error red
\definecolor{cwCd}{HTML}{7A6AB5}
\definecolor{cwOK}{HTML}{548235}     % correct (glyphs)
\definecolor{cwBad}{HTML}{D36265}    % wrong (glyphs, the focal error line)
\definecolor{cwGray}{HTML}{6B6B6B}   % new / unresolved / unknown (strokes, text)
\definecolor{cwInk}{HTML}{222222}
\definecolor{cwNote}{HTML}{5A5A5A}   % secondary text (6.9:1 on white)
\definecolor{cwPanel}{HTML}{F1F3F4}  % the CoWeave band only
\definecolor{cwRule}{HTML}{8F999F}   % dividers (3.0:1 on white)
\definecolor{cwHair}{HTML}{C9CFD3}   % panel separators
\definecolor{cwYel}{HTML}{F0E442}    % annotated person in observed-output figures
\tikzset{
  cw/.style={x=1pt,y=1pt,line cap=round,line join=round,font=\scriptsize,text=cwInk},
  panel/.style={fill=none,draw=none},
  ptitle/.style={anchor=north west,inner sep=0pt,font=\footnotesize\bfseries},
  psub/.style={anchor=north west,inner sep=0pt,font=\scriptsize,text=cwNote},
  plab/.style={inner sep=0pt,font=\scriptsize},
  phead/.style={inner sep=0pt,font=\scriptsize\bfseries},
  pnote/.style={inner sep=0pt,font=\scriptsize\itshape,text=cwNote},
  idn/.style={circle,draw=#1d,line width=0.6pt,shading=radial,inner color=white,outer color=#1!42,minimum size=11.5pt,inner sep=0pt,font=\scriptsize\bfseries,text=#1d!80!black},
  obs/.style={circle,draw=cwInk!75,line width=0.5pt,fill=white,minimum size=11.5pt,inner sep=0pt,font=\scriptsize},
  out/.style={rounded corners=2.5pt,draw=#1d,line width=0.8pt,fill=#1!16,minimum height=10.5pt,minimum width=15pt,inner sep=1.5pt,font=\scriptsize\bfseries,text=#1d},
  newid/.style={rounded corners=2.5pt,draw=cwGray,line width=0.5pt,fill=white,minimum height=10.5pt,minimum width=15pt,inner sep=1.5pt,font=\scriptsize\itshape,text=cwGray},
  unres/.style={rounded corners=2.5pt,draw=cwGray,dash pattern=on 1.6pt off 1.2pt,line width=0.6pt,fill=white,minimum height=10.5pt,minimum width=15pt,inner sep=1.5pt,font=\scriptsize,text=cwGray},
  ctx/.style={draw=cwInk!70,line width=0.5pt,dash pattern=on 2pt off 1.5pt},
  link/.style={draw=cwInk!80,line width=0.8pt},
  cand/.style={draw=cwInk!55,line width=0.5pt},
  flow/.style={draw=cwInk,line width=0.8pt,-{Stealth[length=4pt,width=3.4pt]}},
  thin/.style={draw=cwInk,line width=0.5pt,-{Stealth[length=3pt,width=2.6pt]}},
  tag/.style={fill=white,draw=cwInk!70,line width=0.5pt,inner sep=1pt,font=\scriptsize\bfseries},
  photo/.style={inner sep=0pt,draw=cwInk!45,line width=0.5pt},
  okmark/.style={text=cwOK,font=\footnotesize\bfseries,inner sep=0pt},
  badmark/.style={text=cwBad,font=\footnotesize\bfseries,inner sep=0pt},
  oursband/.style={fill=cwPanel,draw=none},
  hair/.style={draw=cwHair,line width=0.5pt},
}
\newcommand{\cwok}{\ensuremath{\checkmark}}
\newcommand{\cwbad}{\ensuremath{\boldsymbol{\times}}}
\newcommand{\cwown}[6]{%
  \pgfmathsetmacro{\cwoa}{#3*#5}\pgfmathsetmacro{\cwob}{#3*#6}%
  \fill[cwA!80] (#1,#2) rectangle ++(\cwoa,#4);
  \fill[cwB!80] (#1+\cwoa,#2) rectangle ++(\cwob,#4);
  \fill[cwGray!25] (#1+\cwoa+\cwob,#2) rectangle (#1+#3,#2+#4);
  \draw[cwInk!60,line width=0.5pt] (#1,#2) rectangle ++(#3,#4);}
\newcommand{\cwphoto}[7]{\node[photo,anchor=#7] (#1) at (#2,#3) {\includegraphics[width=#4pt,height=#5pt]{figures/tikz/assets/cw/#6}};}
\newcommand{\cwgt}[3]{%
  \edef\cwtmp{\csname cwbox@#2\endcsname}%
  \expandafter\cwgtbody\cwtmp\relax{#1}{#3}}
\def\cwgtbody#1/#2/#3/#4\relax#5#6{%
  \path let \p1=(#5.south west), \p2=(#5.north east) in
    coordinate (cwgt-sw) at ({\x1+#1*(\x2-\x1)},{\y1+#2*(\y2-\y1)})
    coordinate (cwgt-ne) at ({\x1+#3*(\x2-\x1)},{\y1+#4*(\y2-\y1)});
  \draw[#6] (cwgt-sw) rectangle (cwgt-ne);}
\newcommand{\cwfeat}[5]{%
  \foreach \cwv [count=\cwi from 0] in {#5}{\fill[cwInk!\cwv] (#1+\cwi*#3,#2) rectangle ++(#3,#4);}
  \foreach \cwv [count=\cwi from 1] in {#5}{\xdef\cwn{\cwi}}%
  \draw[cwInk!60,line width=0.5pt] (#1,#2) rectangle ++(\cwn*#3,#4);}
\newcommand{\cwmat}[8]{%
  \fill[cwSup!#4] (#1,#2) rectangle ++(#3,#3);   \fill[cwSup!#5] (#1+#3,#2) rectangle ++(#3,#3);
  \fill[cwSup!#6] (#1,#2-#3) rectangle ++(#3,#3); \fill[cwSup!#7] (#1+#3,#2-#3) rectangle ++(#3,#3);
  \draw[cwInk!60,line width=0.5pt] (#1,#2-#3) rectangle ++(2*#3,2*#3) (#1+#3,#2-#3) -- ++(0,2*#3) (#1,#2) -- ++(2*#3,0);
  \ifnum#8>0
    \node[plab,anchor=south,font=\scriptsize\bfseries,text=cwAd] at (#1+0.5*#3,#2+#3+0.5) {A};
    \node[plab,anchor=south,font=\scriptsize\bfseries,text=cwBd] at (#1+1.5*#3,#2+#3+0.5) {B};\fi
  \ifnum#8=1
    \node[plab,anchor=east] at (#1-1,#2+0.5*#3) {$x$};
    \node[plab,anchor=east] at (#1-1,#2-0.5*#3) {$y$};
  \fi}
\tikzset{cam/.pic={
  \path[fill=cwInk!80,rounded corners=0.5pt] (-3.5,-1.6) rectangle (0.9,1.6);
  \path[fill=cwInk!80] (0.9,-0.4) -- (3.5,-1.7) -- (3.5,1.7) -- (0.9,0.4) -- cycle;}}
\newcommand{\cwfov}[6]{%
  \fill[cwInk!10] (#1,#2) -- ++(#3-28:#4) arc[start angle=#3-28,end angle=#3+28,radius=#4] -- cycle;
  \draw[cwInk!35,line width=0.5pt] (#1,#2) -- ++(#3-28:#4) (#1,#2) -- ++(#3+28:#4);
  \pic[rotate=#3] at (#1,#2) {cam};
  \node[plab,font=\scriptsize\bfseries,anchor=#6,outer sep=5pt] at (#1,#2) {#5};}
\newcommand{\cwcam}[2]{%
  \path[fill=cwInk!80,rounded corners=0.6pt] (#1,#2-2.2) rectangle ++(5.6,4.4);
  \path[fill=cwInk!80] (#1+5.6,#2-0.6) -- (#1+8.6,#2-2.2) -- (#1+8.6,#2+2.2) -- (#1+5.6,#2+0.6) -- cycle;}
\newcommand{\cwlock}[2]{%
  \draw[cwInk,line width=0.6pt] (#1-1.6,#2+1.2) -- (#1-1.6,#2+2.6) arc[start angle=180,end angle=0,radius=1.6pt] -- (#1+1.6,#2+1.2);
  \path[fill=white,draw=cwInk,line width=0.6pt,rounded corners=0.5pt] (#1-2.6,#2-2.4) rectangle (#1+2.6,#2+1.4);}
\newcommand{\cwenc}[6]{%
  \path[fill=cwInk!8,draw=cwInk!70,line width=0.6pt,rounded corners=1pt] (#2,#3-#5/2) -- (#2+#4,#3-#6/2) -- (#2+#4,#3+#6/2) -- (#2,#3+#5/2) -- cycle;
  \coordinate (#1-in) at (#2,#3); \coordinate (#1-out) at (#2+#4,#3);}
\definecolor{cwTAmber}{HTML}{FFF1CC} \definecolor{cwLAmber}{HTML}{E2B33C} \definecolor{cwHAmber}{HTML}{FFE699}
\definecolor{cwTGrey}{HTML}{F3F7F9}  \definecolor{cwLGrey}{HTML}{899FA5}  \definecolor{cwHGrey}{HTML}{C4D4DD}
\definecolor{cwTRose}{HTML}{FDF0F3}  \definecolor{cwLRose}{HTML}{D99AB3}  \definecolor{cwHRose}{HTML}{FBDCE0}
\definecolor{cwTGreen}{HTML}{E8F3E2} \definecolor{cwLGreen}{HTML}{8DBF6E}  \definecolor{cwHGreen}{HTML}{C7E4B3}
\definecolor{cwTBad}{HTML}{FDF0F3}   \definecolor{cwLBad}{HTML}{D36265}   \definecolor{cwHBad}{HTML}{FBDCE0}
\definecolor{cwTGood}{HTML}{E8F3E2}  \definecolor{cwLGood}{HTML}{8DBF6E}  \definecolor{cwHGood}{HTML}{C7E4B3}
\definecolor{cwHi}{HTML}{FFE699}     \definecolor{cwHiD}{HTML}{BF9000}    % key-claim highlight (yellow)
\definecolor{cwSup}{HTML}{8C8CE0}    \definecolor{cwSupL}{HTML}{CECEFA}   % support / score (lavender ramp)
\definecolor{cwTokA}{HTML}{99CCFF} \definecolor{cwTokB}{HTML}{C7E4B3} \definecolor{cwTokC}{HTML}{FFE699} \definecolor{cwTokD}{HTML}{CECEFA}
\definecolor{cwTSky}{HTML}{E4F6FC} \definecolor{cwLSky}{HTML}{9DC3E6} \definecolor{cwHSky}{HTML}{DDEAF7}
\definecolor{cwGold}{HTML}{FFC000} \definecolor{cwGoldL}{HTML}{FFF1C9} \definecolor{cwPeach}{HTML}{F8CAAC}
\definecolor{cwGlass}{HTML}{E4F6FC} \definecolor{cwGlassL}{HTML}{A8CFE8}
\definecolor{cwFeat}{HTML}{55636F}
\newcommand{\cwbadge}[1]{\tikz[baseline=-0.62ex]\node[circle,fill=cwInk,text=white,inner sep=0pt,minimum size=8.4pt,font=\scriptsize\bfseries] {#1};}
\newcommand{\cwbox}[7]{%
  \path[fill=cwT#5,draw=cwL#5,line width=0.75pt,dash pattern=on 2.6pt off 1.7pt,rounded corners=4pt] (#1,#2) rectangle (#3,#4);
  \node[anchor=west,inner sep=0pt,font=\footnotesize\bfseries\itshape,text=cwInk] at (#1+4,#4-7.2) {\cwbadge{#6}\,\,#7};}
\newcommand{\cwtab}[6]{%
  \path[fill=cwH#5,draw=cwL#5,line width=0.6pt,rounded corners=3pt] (#1,#2) rectangle (#3,#4);
  \node[align=center,inner sep=0pt,font=\scriptsize\bfseries,text=cwInk] at ({(#1+#3)/2},{(#2+#4)/2}) {#6};}
\newcommand{\cwplate}[5]{%
  \path[fill=cwL#5!70,rounded corners=1pt] (#1,#3-#4/2-1.6) -- (#2,#3-#4/2-1.6) -- (#2+7,#3+#4/2-1.6) -- (#1+7,#3+#4/2-1.6) -- cycle;
  \path[fill=cwH#5,draw=cwL#5,line width=0.5pt,rounded corners=1pt] (#1,#3-#4/2) -- (#2,#3-#4/2) -- (#2+7,#3+#4/2) -- (#1+7,#3+#4/2) -- cycle;}
\newcommand{\cwtok}[5]{%
  \foreach \cwi in {1,...,#3}{\foreach \cwj in {1,...,#4}{
    \pgfmathtruncatemacro{\cwlv}{mod(\cwi*37+\cwj*53,50)+12}
    \pgfmathtruncatemacro{\cwtk}{mod(\cwi+2*\cwj,4)}%
    \ifcase\cwtk\def\cwtc{cwTokA}\or\def\cwtc{cwTokB}\or\def\cwtc{cwTokC}\else\def\cwtc{cwTokD}\fi
    \path[fill=\cwtc,draw=cwInk!55,line width=0.35pt] (#1+\cwi*#5-#5,#2-\cwj*#5) rectangle ++(#5,#5);}}
  \draw[cwInk!70,line width=0.5pt] (#1,#2-#4*#5) rectangle (#1+#3*#5,#2);}
\newcommand{\cwfilm}[4]{%
  \path[fill=cwInk!88,rounded corners=1.5pt] (#1,#2) rectangle (#3,#4);
  \pgfmathsetmacro{\cwfn}{floor((#3-#1-4)/6)}
  \foreach \cwk in {0,...,\cwfn}{\path[fill=white] (#1+3+\cwk*6,#2+1.1) rectangle ++(2.6,1.9);
    \path[fill=white] (#1+3+\cwk*6,#4-3) rectangle ++(2.6,1.9);}}
\tikzset{pill/.style={fill=cwGoldL,draw=cwHiD,line width=0.5pt,rounded corners=3pt,inner xsep=3pt,inner ysep=1.6pt,font=\scriptsize\itshape}}
\def\cwdx{0.55}\def\cwdy{0.42}
\newcommand{\cwslab}[6]{%
  \colorlet{cwslabt}{#5}\colorlet{cwslabe}{#6}%
  \pgfmathsetmacro{\cwsx}{#4*\cwdx}\pgfmathsetmacro{\cwsy}{#4*\cwdy}%
  \path[fill=cwslabe!55,blur shadow={shadow blur steps=6,shadow xshift=1.2pt,shadow yshift=-1.6pt,shadow opacity=25}]
     (#1,#2-3) -- (#1+#3,#2-3) -- (#1+#3+\cwsx,#2+\cwsy-3) -- (#1+#3+\cwsx,#2+\cwsy) -- (#1+\cwsx,#2+\cwsy) -- (#1,#2) -- cycle;
  \path[fill=cwslabe!70] (#1,#2-3) rectangle (#1+#3,#2);
  \path[fill=cwslabe!45] (#1+#3,#2-3) -- (#1+#3+\cwsx,#2+\cwsy-3) -- (#1+#3+\cwsx,#2+\cwsy) -- (#1+#3,#2) -- cycle;
  \path[top color=cwslabt!55,bottom color=cwslabt,draw=cwslabe,line width=0.5pt]
     (#1,#2) -- (#1+#3,#2) -- (#1+#3+\cwsx,#2+\cwsy) -- (#1+\cwsx,#2+\cwsy) -- cycle;}
\newcommand{\cwflat}[6]{%
  \begin{scope}[shift={(#2,#3)},cm={1,0,\cwdx,\cwdy,(0,0)}]
    \node[inner sep=0pt,anchor=south west,transform shape] (#1) at (0,0) {\includegraphics[width=#4pt,height=#5pt]{figures/tikz/assets/cw/#6}};
    \draw[white,line width=0.8pt] (0,0) rectangle (#4,#5);
    \coordinate (#1-c) at (#4/2,#5/2); \coordinate (#1-fl) at (0,0); \coordinate (#1-fr) at (#4,0);
    \coordinate (#1-bl) at (0,#5); \coordinate (#1-br) at (#4,#5);
  \end{scope}}
\newcommand{\cwcube}[4]{%
  \colorlet{cwcubec}{#4}%
  \pgfmathsetmacro{\cwcx}{#3*0.5*\cwdx}\pgfmathsetmacro{\cwcy}{#3*0.5*\cwdy}%
  \path[fill=cwcubec!55!white,draw=cwcubec!55!black,line width=0.3pt] (#1,#2+#3) -- ++(\cwcx,\cwcy) -- ++(#3,0) -- ++(-\cwcx,-\cwcy) -- cycle;
  \path[fill=cwcubec!80!black,draw=cwcubec!55!black,line width=0.3pt] (#1+#3,#2) -- ++(\cwcx,\cwcy) -- ++(0,#3) -- ++(-\cwcx,-\cwcy) -- cycle;
  \path[fill=cwcubec,draw=cwcubec!55!black,line width=0.3pt] (#1,#2) rectangle ++(#3,#3);}
\newcommand{\cwbar}[6]{%
  \colorlet{cwbarc}{#6}%
  \pgfmathsetmacro{\cwbx}{#4*\cwdx}\pgfmathsetmacro{\cwby}{#4*\cwdy}%
  \path[fill=cwbarc!80!black,draw=cwbarc!50!black,line width=0.35pt] (#1+#3,#2) -- ++(\cwbx,\cwby) -- ++(0,#5) -- ++(-\cwbx,-\cwby) -- cycle;
  \path[fill=cwbarc!45!white,draw=cwbarc!50!black,line width=0.35pt] (#1,#2+#5) -- ++(\cwbx,\cwby) -- ++(#3,0) -- ++(-\cwbx,-\cwby) -- cycle;
  \path[fill=cwbarc,draw=cwbarc!50!black,line width=0.35pt] (#1,#2) rectangle ++(#3,#5);}
\tikzset{
  card/.style={inner sep=0pt,draw=white,line width=0.8pt,blur shadow={shadow blur steps=5,shadow xshift=1pt,shadow yshift=-1.2pt,shadow opacity=35}},
  beam/.style={fill=cwHi,opacity=0.42},
  glow/.style={draw=cwHiD,line width=1.1pt},
}
\newcommand{\cwring}[6]{%
  \pgfmathsetmacro{\cwra}{90-360*#4}\pgfmathsetmacro{\cwrb}{\cwra-360*#5}%
  \draw[cwGray!25,line width=#6] (#1,#2) circle[radius=#3];
  \draw[cwA,line width=#6,line cap=butt] (#1,#2) ++(90:#3) arc[start angle=90,end angle=\cwra,radius=#3];
  \draw[cwB,line width=#6,line cap=butt] (#1,#2) ++(\cwra:#3) arc[start angle=\cwra,end angle=\cwrb,radius=#3];
  \draw[white,line width=0.3pt] (#1,#2) circle[radius=#3+#6/2] (#1,#2) circle[radius=#3-#6/2];}
\newcommand{\cwspark}[3]{%
  \foreach \cwang in {0,45,...,315}{\draw[cwGold,line width=0.6pt] (#1,#2) ++(\cwang:#3*0.35) -- ++(\cwang:#3*0.65);}
  \fill[cwGold] (#1,#2) circle[radius=#3*0.18];}
\newcommand{\cwgauge}[5]{%
  \foreach \cwg in {1,...,#4}{%
    \pgfmathsetmacro{\cwga}{180-(\cwg-1)*180/#4-2}\pgfmathsetmacro{\cwgb}{180-\cwg*180/#4+2}%
    \ifnum\cwg>#5 \def\cwgc{cwHGrey}\else\def\cwgc{cwAd}\fi
    \draw[\cwgc,line width=4.2pt,line cap=butt] (#1,#2) ++(\cwga:#3) arc[start angle=\cwga,end angle=\cwgb,radius=#3];}
  \draw[cwInk,line width=0.7pt,-{Stealth[length=3pt]}] (#1,#2) -- ++({180-#5*180/#4}:#3-4);
  \fill[cwInk] (#1,#2) circle[radius=1.4pt];}
\tikzset{
  glowA/.style={draw=cwA,line width=4.2pt,opacity=0.22,line cap=round},
  glowB/.style={draw=cwB,line width=4.2pt,opacity=0.25,line cap=round},
  glowG/.style={draw=cwGold,line width=4.2pt,opacity=0.3,line cap=round},
  gold/.style={draw=cwGold,line width=1.2pt},
  poison/.style={left color=cwBad!8,right color=cwBad!45},
}
\definecolor{cwOurs}{HTML}{4F46A5}\definecolor{cwOursL}{HTML}{DEDCF3}\definecolor{cwOursM}{HTML}{A7A2DB}% CoWeave: indigo, the hue of Fig. 2 (4)
\newcommand{\cwpcard}[5]{%
  \path[fill=cwInk!3.5,rounded corners=4pt] (#1,#2) rectangle (#3,#4);
  \node[anchor=north west,inner sep=0pt,font=\footnotesize\bfseries,text=cwInk] at (#1+5,#4-4.5) {#5};}
\tikzset{sc/.style={inner sep=0pt,font=\fontsize{7.4}{8.4}\selectfont\scshape,text=cwNote}}
\pgfplotsset{/tikz/fill between/on layer=main}
\definecolor{cwB1}{HTML}{4F565F}\definecolor{cwB2}{HTML}{7E848C}\definecolor{cwB3}{HTML}{A2A7AE}\definecolor{cwB4}{HTML}{C3C7CC}\definecolor{cwL3}{HTML}{8A9098}\definecolor{cwL4}{HTML}{A6ABB2}% plot lines
\pgfplotsset{cw axis/.style={%
  scale only axis, axis lines=left, axis line style={cwInk!65,line width=0.5pt,-},%
  every tick/.style={cwInk!65,line width=0.45pt}, tick align=outside, major tick length=2pt,%
  tick label style={font=\footnotesize,text=cwInk}, label style={font=\footnotesize,text=cwInk},%
  xlabel style={yshift=2.6pt}, ylabel style={yshift=-3pt},%
  ymajorgrids, every axis grid/.style={}, grid style={cwInk!9,line width=0.45pt,-}, clip mode=individual}}
\input{figures/tikz/supp_cw_boxes}
