# Supplementary material for: CoWeave: Identity-Specific Context Reasoning for Persistent Multi-Camera Tracking
Source: arXiv:2611.38993 source file (2026-11-28)
Supplement: Supplementary file 2 [file supp_cw_boxes.tex]

\expandafter\def\csname cwbox@m_c03_1370-A\endcsname{0.1218/0.0536/0.3959/0.7739}%
\expandafter\def\csname cwbox@m_c03_1370-B\endcsname{0.6467/0.1597/0.8782/0.9464}%
\expandafter\def\csname cwbox@m_c08_1011-A\endcsname{0.2261/0.0207/0.3997/0.6919}%
\expandafter\def\csname cwbox@m_c08_1011-B\endcsname{0.3598/0.3260/0.4725/0.9136}%
\expandafter\def\csname cwbox@m_c12_5544-A\endcsname{0.3215/0.0199/0.5252/0.8770}%
\expandafter\def\csname cwbox@m_c12_5544-B\endcsname{0.4269/0.0040/0.6883/0.7499}%
\expandafter\def\csname cwbox@m_c03_1433-A\endcsname{0.3659/0.2538/0.5379/0.8225}%
\expandafter\def\csname cwbox@m_c03_1433-B\endcsname{0.5472/0.0040/0.7034/0.5468}%
\expandafter\def\csname cwbox@m_c08_1068-A\endcsname{0.3598/0.1726/0.6402/0.8145}%
\expandafter\def\csname cwbox@m_c08_1068-B\endcsname{0.4768/0.5128/0.5973/0.9960}%
\expandafter\def\csname cwbox@o_A_c04_92-C\endcsname{0.1875/-0.7534/0.8808/0.9363}%
\expandafter\def\csname cwbox@o_A_c04_92_ctx-C\endcsname{0.4544/0.2397/0.5556/0.6886}%
\expandafter\def\csname cwbox@o_A_c04_92_ctx-P\endcsname{0.4445/0.3087/0.5555/0.6913}%
\expandafter\def\csname cwbox@o_A_c04_345-C\endcsname{0.1429/-0.4999/0.8202/0.9700}%
\expandafter\def\csname cwbox@o_A_c04_345_ctx-C\endcsname{0.1002/0.4935/0.1905/0.8506}%
\expandafter\def\csname cwbox@o_A_c04_345_ctx-P\endcsname{0.1049/0.4950/0.1907/0.8449}%
\expandafter\def\csname cwbox@o_A_c02_345-C\endcsname{0.1593/-0.4834/0.8023/0.8970}%
\expandafter\def\csname cwbox@o_A_c02_345_ctx-C\endcsname{0.4568/0.3361/0.5383/0.6549}%
\expandafter\def\csname cwbox@o_A_c02_345_ctx-P\endcsname{0.4601/0.3337/0.5399/0.6663}%
\expandafter\def\csname cwbox@o_A_c02_368-C\endcsname{0.1447/-0.5160/0.8417/0.9030}%
\expandafter\def\csname cwbox@o_A_c02_368_ctx-C\endcsname{0.4521/0.3176/0.5461/0.6662}%
\expandafter\def\csname cwbox@o_A_c02_368_ctx-P\endcsname{0.4552/0.3231/0.5448/0.6769}%
\expandafter\def\csname cwbox@o_B_c02_575-C\endcsname{0.1131/0.0000/0.9791/0.5347}%
\expandafter\def\csname cwbox@o_B_c02_575_ctx-C\endcsname{0.4278/0.0000/0.5894/0.1818}%
\expandafter\def\csname cwbox@o_B_c02_575_ctx-P\endcsname{0.4167/0.0040/0.5833/0.1787}%
\expandafter\def\csname cwbox@o_B_c03_1380-M\endcsname{-0.2882/-0.1745/1.0835/1.0168}%
\expandafter\def\csname cwbox@o_B_c03_1380-C\endcsname{0.0495/-0.3088/0.9155/0.9269}%
\expandafter\def\csname cwbox@o_B_c03_1380_ctx-M\endcsname{0.1747/0.2826/0.4759/0.7591}%
\expandafter\def\csname cwbox@o_B_c03_1380_ctx-C\endcsname{0.2489/0.2289/0.4391/0.7232}%
\expandafter\def\csname cwbox@o_B_c03_1380_ctx-P\endcsname{0.2498/0.2265/0.4458/0.7231}%
\expandafter\def\csname cwbox@o_B_c03_1403-M\endcsname{-0.0054/-0.1653/0.9196/0.9651}%
\expandafter\def\csname cwbox@o_B_c03_1403-C\endcsname{0.1799/-0.4914/0.8237/0.9487}%
\expandafter\def\csname cwbox@o_B_c03_1403_ctx-M\endcsname{0.3614/0.4013/0.5655/0.8555}%
\expandafter\def\csname cwbox@o_B_c03_1403_ctx-C\endcsname{0.4023/0.2703/0.5443/0.8489}%
\expandafter\def\csname cwbox@o_B_c03_1403_ctx-P\endcsname{0.4041/0.2694/0.5417/0.8480}%
\expandafter\def\csname cwbox@o_B_c03_1449-M\endcsname{0.0275/-0.2586/0.8829/1.0713}%
\expandafter\def\csname cwbox@o_B_c03_1449-C\endcsname{0.1108/0.0479/0.7332/0.9472}%
\expandafter\def\csname cwbox@o_B_c03_1449_ctx-M\endcsname{0.4037/0.2921/0.5780/0.7858}%
\expandafter\def\csname cwbox@o_B_c03_1449_ctx-C\endcsname{0.4207/0.4059/0.5475/0.7397}%
\expandafter\def\csname cwbox@o_B_c03_1449_ctx-P\endcsname{0.4241/0.2049/0.5759/0.7394}%
\expandafter\def\csname cwbox@o_C_c05_1104-C\endcsname{0.1629/-0.4946/0.7914/0.9710}%
\expandafter\def\csname cwbox@o_C_c05_1104_ctx-C\endcsname{0.4616/0.3842/0.5332/0.6879}%
\expandafter\def\csname cwbox@o_C_c05_1104_ctx-P\endcsname{0.4696/0.3844/0.5304/0.6828}%
\expandafter\def\csname cwbox@o_C_c01_1127-C\endcsname{0.1419/-0.4560/0.8674/0.9484}%
\expandafter\def\csname cwbox@o_C_c01_1127_ctx-C\endcsname{0.4478/0.3187/0.5536/0.6918}%
\expandafter\def\csname cwbox@o_C_c01_1127_ctx-P\endcsname{0.4471/0.3087/0.5529/0.6913}%
\expandafter\def\csname cwbox@o_C_c01_1150-C\endcsname{0.1869/-0.4644/0.8131/0.9476}%
\expandafter\def\csname cwbox@o_C_c01_1150_ctx-C\endcsname{0.4543/0.3165/0.5457/0.6917}%
\expandafter\def\csname cwbox@o_C_c01_1150_ctx-P\endcsname{0.4516/0.3087/0.5484/0.6913}%
\expandafter\def\csname cwbox@o_C_c01_1449_ctx-P\endcsname{0.4742/0.4355/0.5257/0.6361}%
\expandafter\def\csname cwbox@o_D_c03_1127-M\endcsname{0.0040/0.2005/1.0624/1.0692}%
\expandafter\def\csname cwbox@o_D_c03_1127-C\endcsname{0.0576/0.2360/0.9476/0.9259}%
\expandafter\def\csname cwbox@o_D_c03_1127_ctx-M\endcsname{0.5368/0.1589/0.7822/0.5257}%
\expandafter\def\csname cwbox@o_D_c03_1127_ctx-C\endcsname{0.5492/0.1739/0.7556/0.4652}%
\expandafter\def\csname cwbox@o_D_c03_1127_ctx-P\endcsname{0.5483/0.0040/0.7553/0.4656}%
\expandafter\def\csname cwbox@o_D_c03_1150-M\endcsname{0.0687/0.1345/1.0843/1.0105}%
\expandafter\def\csname cwbox@o_D_c03_1150-C\endcsname{0.0831/0.0224/0.9508/0.9161}%
\expandafter\def\csname cwbox@o_D_c03_1150_ctx-M\endcsname{0.4979/0.0650/0.7673/0.4882}%
\expandafter\def\csname cwbox@o_D_c03_1150_ctx-C\endcsname{0.5017/0.0108/0.7318/0.4426}%
\expandafter\def\csname cwbox@o_D_c03_1150_ctx-P\endcsname{0.4939/0.0040/0.7307/0.4459}%
\expandafter\def\csname cwbox@o_D_c03_1173-M\endcsname{0.0024/0.0040/1.2475/0.8166}%
\expandafter\def\csname cwbox@o_D_c03_1173-C\endcsname{0.0386/0.0142/0.9655/0.7681}%
\expandafter\def\csname cwbox@o_D_c03_1173_ctx-M\endcsname{0.4412/0.0021/0.8007/0.4295}%
\expandafter\def\csname cwbox@o_D_c03_1173_ctx-C\endcsname{0.4516/0.0075/0.7193/0.4040}%
\expandafter\def\csname cwbox@o_D_c03_1173_ctx-P\endcsname{0.4559/0.0040/0.7138/0.4008}%
\expandafter\def\csname cwbox@o_D_c03_1196-M\endcsname{0.0559/0.0089/1.1881/0.6791}%
\expandafter\def\csname cwbox@o_D_c03_1196-C\endcsname{0.1004/0.0043/0.9603/0.6096}%
\expandafter\def\csname cwbox@o_D_c03_1196_ctx-M\endcsname{0.3998/0.0047/0.7316/0.3625}%
\expandafter\def\csname cwbox@o_D_c03_1196_ctx-C\endcsname{0.4128/0.0023/0.6648/0.3254}%
\expandafter\def\csname cwbox@o_D_c03_1196_ctx-P\endcsname{0.3991/0.0040/0.6608/0.3284}%
