# Supplementary material for: CoWeave: Identity-Specific Context Reasoning for Persistent Multi-Camera Tracking
Source: arXiv:2611.38993 source file (2026-11-28)
Supplement: Supplementary file 3 [file supp_control_readings.tex]

\newcommand{\RepairEver}{\pv{75}}
\newcommand{\RepairMedian}{\pv{5}}
\newcommand{\RepairHeld}{\pv{69}}
\newcommand{\RepairLost}{\pv{6}}
\newcommand{\RepairNever}{\pv{25}}
\newcommand{\RepairHeldPct}{\pv{92}}
\newcommand{\RetentionCo}{\pv{80.5}}
\newcommand{\RetentionBest}{\pv{72.7}}
\newcommand{\RetentionMargin}{\pv{7.8}}
