# Supplementary material for: CoWeave: Identity-Specific Context Reasoning for Persistent Multi-Camera Tracking
Source: arXiv:2611.38993 source file (2026-11-28)
Supplement: Supplementary file 4 [file supp_numbers.tex]

\newcommand{\GoalID}{\pv{80.5}}
\newcommand{\BaseID}{\pv{72.9}}
\newcommand{\DeltaID}{\pv{7.6}}
\newcommand{\GoalC}{\pv{86.5}}
\newcommand{\BaseC}{\pv{77.8}}
\newcommand{\GoalW}{\pv{2.5}}
\newcommand{\BaseW}{\pv{5.9}}
\newcommand{\IndepW}{\pv{9.0}}
\newcommand{\GoalN}{\pv{11.0}}
\newcommand{\BaseN}{\pv{16.3}}
\newcommand{\GoalP}{\pv{82.1}}
\newcommand{\BaseP}{\pv{67.0}}
\newcommand{\DeltaP}{\pv{15.1}}
\newcommand{\LeadZero}{\pv{8.7}}
\newcommand{\Wdelta}{\pv{3.4}}
\newcommand{\Wrelative}{\pv{57.6}}
\newcommand{\WrongMin}{\pv{5.9}}
\newcommand{\WrongMax}{\pv{8.3}}
\newcommand{\TimeDelta}{\pv{8.4}}
\newcommand{\GoalMs}{\pv{46.6}}
\newcommand{\BaseMs}{\pv{43.0}}
\newcommand{\MctrMs}{\pv{49.8}}
\newcommand{\InitShare}{\pv{7.9}}
\newcommand{\RetShare}{\pv{7.2}}
\newcommand{\InitPct}{\pv{52}}
\newcommand{\ReaderGain}{\pv{7.1}}
\newcommand{\MatcherGain}{\pv{7.3}}
\newcommand{\BothGain}{\pv{15.8}}
\newcommand{\InteractionP}{\pv{1.3}}
\newcommand{\InteractionPlo}{\pv{$-$1.6}}
\newcommand{\InteractionPhi}{\pv{4.2}}
\newcommand{\Interaction}{\pv{0.9}}
\newcommand{\InteractionLo}{\pv{$-$1.2}}
\newcommand{\InteractionHi}{\pv{2.9}}
\newcommand{\ReaderGainH}{\pv{3.2}}
\newcommand{\MatcherGainH}{\pv{3.6}}
\newcommand{\TransferMin}{\pv{4.6}}
\newcommand{\TransferMax}{\pv{7.4}}
\newcommand{\TransferPMin}{\pv{9.7}}
\newcommand{\TransferPMax}{\pv{15.6}}
\newcommand{\Arrivals}{\pv{10,783}}
\newcommand{\Complete}{\pv{8,647}}
\newcommand{\Episodes}{\pv{30}}
\newcommand{\BudgetShift}{\pv{3.9}}
\newcommand{\BudgetCap}{\pv{32}}
\newcommand{\CoScored}{\pv{7.2}}
\newcommand{\InScored}{\pv{3.3}}
\newcommand{\NativeCo}{\pv{82.1}}
\newcommand{\NativeGmt}{\pv{74.9}}
\newcommand{\NativeDelta}{\pv{7.2}}
\newcommand{\NativeDeltaP}{\pv{14.2}}
\newcommand{\AblFixedRet}{\pv{4.3}}
\newcommand{\AblInstance}{\pv{8.7}}
\newcommand{\AblFixedRetID}{\pv{1.3}}
\newcommand{\AblInstanceID}{\pv{6.1}}
\newcommand{\PermCost}{\pv{5.1}}
\newcommand{\ZeroCost}{\pv{5.1}}
\newcommand{\RetMarginID}{\pv{7.8}}
\newcommand{\RetBestID}{\pv{diverse}}
\newcommand{\RetMarginP}{\pv{11.7}}
\newcommand{\RetBestP}{\pv{task-aware independent}}
\newcommand{\SweepMinID}{\pv{77.0}}
\newcommand{\SweepMinP}{\pv{77.0}}
\newcommand{\RevGranoID}{\pv{78.6}}
\newcommand{\RevGranoW}{\pv{3.1}}
\newcommand{\RevGranoP}{\pv{78.4}}
\newcommand{\RevGran}{\pv{3.7}}
\newcommand{\RevGranID}{\pv{1.9}}
\newcommand{\SymArrivals}{\pv{431}}
\newcommand{\SymEpisodes}{\pv{7}}
\newcommand{\TransWcMin}{\pv{3.1}}
\newcommand{\TransWcMax}{\pv{4.0}}
\newcommand{\TransWgMin}{\pv{7.0}}
\newcommand{\TransWgMax}{\pv{7.8}}
\newcommand{\StoreSave}{\pv{6}}
\newcommand{\TransHMin}{\pv{4.9}}
\newcommand{\TransHMax}{\pv{6.8}}
\newcommand{\TransRcMin}{\pv{91.2}}
\newcommand{\TransRcMax}{\pv{93.2}}
\newcommand{\TransRgMin}{\pv{83.1}}
\newcommand{\TransRgMax}{\pv{85.1}}
\newcommand{\ReaderMs}{\pv{44.5}}
\newcommand{\TrackletMs}{\pv{45.2}}
\newcommand{\LeadReliable}{\pv{5.9}}
\newcommand{\LeadGroup}{\pv{19.4}}
\newcommand{\LeadSplit}{\pv{24.6}}
\newcommand{\LeadInvalid}{\pv{31.6}}
\newcommand{\QuarterCo}{\pv{74.2}}
\newcommand{\QuarterCoP}{\pv{71.4}}
\newcommand{\DoubleGmt}{\pv{74.2}}
\newcommand{\InvLossCo}{\pv{2.9}}
\newcommand{\InvLossGmt}{\pv{7.1}}
\newcommand{\SdMax}{\pv{0.8}}
