# Supplementary material for: CoWeave: Identity-Specific Context Reasoning for Persistent Multi-Camera Tracking
Source: arXiv:2611.38993 source file (2026-11-28)
Supplement: Supplementary file 5 [file supp_rowmacros.tex]

\def\RowsMainwide{%
Independent & \pv{68.8} & \pv{57.5} & \pv{68.4} & \pv{9.0} & \pv{22.6} & \pv{55.3} &  & \pv{40.2} & \pv{1.00} &  & \pv{65.0} & \pv{50.7} &  & \pv{61.9} & \pv{47.7} &  & \pv{58.5} & \pv{44.6} \\
DyGLIP & \pv{71.3} & \pv{59.0} & \pv{70.3} & \pv{8.3} & \pv{21.4} & \pv{58.6} &  & \pv{39.5} & \pv{0.99} &  & \pv{67.9} & \pv{54.3} &  & \pv{63.9} & \pv{51.6} &  & \pv{61.0} & \pv{47.2} \\
ReST & \pv{72.1} & \pv{60.9} & \pv{72.7} & \pv{7.6} & \pv{19.8} & \pv{62.2} &  & \pv{37.5} & \pv{0.88} &  & \pv{68.4} & \pv{59.1} &  & \pv{65.8} & \pv{55.4} &  & \pv{61.8} & \pv{51.6} \\
MCTR & \pv{72.7} & \tsecond{\pv{62.7}} & \pv{74.5} & \pv{6.5} & \pv{18.9} & \pv{64.2} &  & \pv{49.8} & \pv{0.71} &  & \pv{69.1} & \pv{58.9} &  & \pv{66.1} & \pv{56.2} &  & \pv{62.6} & \pv{54.6} \\
GMT (causal) & \tsecond{\pv{72.9}} & \pv{62.6} & \tsecond{\pv{77.8}} & \tsecond{\pv{5.9}} & \tsecond{\pv{16.3}} & \tsecond{\pv{67.0}} &  & \pv{43.0} & \pv{1.00} &  & \tsecond{\pv{70.2}} & \tsecond{\pv{63.5}} &  & \tsecond{\pv{66.6}} & \tsecond{\pv{59.9}} &  & \tsecond{\pv{63.1}} & \tsecond{\pv{56.0}} \\
\rowcolor{tabours}\textbf{CoWeave} & \tbest{\pv{80.5}} & \tbest{\pv{69.3}} & \tbest{\pv{86.5}} & \tbest{\pv{2.5}} & \tbest{\pv{11.0}} & \tbest{\pv{82.1}} &  & \pv{46.6} & \pv{0.94} &  & \tbest{\pv{74.8}} & \tbest{\pv{73.2}} &  & \tbest{\pv{74.0}} & \tbest{\pv{75.5}} &  & \tbest{\pv{69.3}} & \tbest{\pv{68.3}} \\
$\Delta$ & \dgood{\pv{$+$7.6}}\dci{\pv{1.1}} & \dgood{\pv{$+$6.7}} & \dgood{\pv{$+$8.7}}\dci{\pv{1.5}} & \dgood{\pv{$-$3.4}}\dci{\pv{0.3}} & \dgood{\pv{$-$5.3}} & \dgood{\pv{$+$15.1}}\dci{\pv{1.8}} &  & \tna & \tna &  & \dgood{\pv{$+$4.6}}\dci{\pv{1.1}} & \dgood{\pv{$+$9.7}} &  & \dgood{\pv{$+$7.4}}\dci{\pv{0.5}} & \dgood{\pv{$+$15.6}} &  & \dgood{\pv{$+$6.2}}\dci{\pv{1.5}} & \dgood{\pv{$+$12.3}} \\%
}
\def\RowsFrontend{%
Independent & \pv{70.1} & \pv{57.1} & \pv{1.00} \\
DyGLIP & \pv{73.1} & \pv{61.0} & \pv{1.17} \\
ReST & \pv{73.7} & \pv{64.3} & \pv{1.06} \\
MCTR & \pv{74.1} & \pv{66.2} & \pv{1.39} \\
GMT (causal) & \tsecond{\pv{74.9}} & \tsecond{\pv{69.8}} & \pv{1.26} \\
\rowcolor{tabours}\textbf{CoWeave} & \tbest{\pv{82.1}} & \tbest{\pv{84.0}} & \pv{1.34} \\
$\Delta$ & \dgood{\pv{$+$7.2}} & \dgood{\pv{$+$14.2}} &  \\%
}
\def\RowsAblationmain{%
\rowcolor{tabgroup}\multicolumn{5}{l}{\textit{\textbf{Single-part replacement, same read budget}}} \\
\rowcolor{tabours}\textbf{Full CoWeave} & \tbest{\pv{80.5}} & \tbest{\pv{2.5}} & \tbest{\pv{82.1}} & \tna \\
Fixed retrieval & \pv{79.2} & \pv{3.3} & \pv{77.8} & \dbad{\pv{$-$4.3}} \\
Zero relational support & \pv{77.1} & \pv{3.5} & \pv{77.0} & \dbad{\pv{$-$5.1}} \\
Tracklet-level reassignment & \pv{78.6} & \pv{3.1} & \pv{78.4} & \dbad{\pv{$-$3.7}} \\
Fixed record ownership & \pv{76.5} & \pv{3.8} & \pv{74.9} & \dbad{\pv{$-$7.2}} \\
Without instance detail & \pv{74.4} & \pv{4.5} & \pv{73.4} & \dbad{\pv{$-$8.7}} \\
\rowcolor{tabgroup}\multicolumn{5}{l}{\textit{\textbf{Retention policy, same storage cap}}} \\
\rowcolor{tabours}\textbf{Full CoWeave} & \tbest{\pv{80.5}} & \tbest{\pv{2.5}} & \tbest{\pv{82.1}} & \tna \\
Recent & \pv{72.1} & \pv{6.9} & \pv{65.8} & \dbad{\pv{$-$16.3}} \\
Diverse & \pv{72.7} & \pv{6.5} & \pv{68.4} & \dbad{\pv{$-$13.7}} \\
Task-aware independent & \pv{72.1} & \pv{5.8} & \pv{70.4} & \dbad{\pv{$-$11.7}} \\%
}
\def\StyIdcounts{%
Independent & \pv{896,394} & \pv{424,703} & \pv{388,762} & \pv{67.9} & \pv{69.8} & \pv{68.8} \\
DyGLIP & \pv{934,865} & \pv{403,387} & \pv{350,291} & \pv{69.9} & \pv{72.7} & \pv{71.3} \\
ReST & \pv{919,019} & \tsecond{\pv{346,670}} & \pv{366,137} & \tsecond{\pv{72.6}} & \pv{71.5} & \pv{72.1} \\
MCTR & \pv{940,455} & \pv{362,296} & \pv{344,700} & \pv{72.2} & \tsecond{\pv{73.2}} & \pv{72.7} \\
GMT (causal) & \tsecond{\pv{941,320}} & \pv{355,372} & \tsecond{\pv{343,836}} & \tsecond{\pv{72.6}} & \tsecond{\pv{73.2}} & \tsecond{\pv{72.9}} \\
\rowcolor{tabours}\textbf{CoWeave} (ours) & \tbest{\pv{1,030,925}} & \tbest{\pv{245,567}} & \tbest{\pv{254,230}} & \tbest{\pv{80.8}} & \tbest{\pv{80.2}} & \tbest{\pv{80.5}} \\
$\Delta$ & \dgood{\pv{$+$89,605}} & \dgood{\pv{$-$109,805}} & \dgood{\pv{$-$89,606}} & \dgood{\pv{$+$8.2}} & \dgood{\pv{$+$7.0}} & \dgood{\pv{$+$7.6}} \\%
}
\def\StySeeds{%
Independent & \pv{68.8}\dci{\pv{0.13}} & \pv{57.5}\dci{\pv{0.25}} & \pv{68.4}\dci{\pv{0.33}} & \pv{9.0}\dci{\pv{0.18}} & \pv{22.6}\dci{\pv{0.48}} & \pv{55.3}\dci{\pv{0.33}} & \pv{80.9}\dci{\pv{0.32}} \\
DyGLIP & \pv{71.3}\dci{\pv{0.76}} & \pv{59.0}\dci{\pv{0.55}} & \pv{70.3}\dci{\pv{0.25}} & \pv{8.3}\dci{\pv{0.01}} & \pv{21.4}\dci{\pv{0.26}} & \pv{58.6}\dci{\pv{0.19}} & \pv{83.3}\dci{\pv{0.30}} \\
ReST & \pv{72.1}\dci{\pv{0.62}} & \pv{60.9}\dci{\pv{0.20}} & \pv{72.7}\dci{\pv{0.21}} & \pv{7.6}\dci{\pv{0.01}} & \pv{19.8}\dci{\pv{0.22}} & \pv{62.2}\dci{\pv{0.50}} & \pv{85.6}\dci{\pv{0.82}} \\
MCTR & \pv{72.7}\dci{\pv{0.53}} & \pv{62.7}\dci{\pv{0.62}} & \pv{74.5}\dci{\pv{0.49}} & \pv{6.5}\dci{\pv{0.10}} & \pv{18.9}\dci{\pv{0.50}} & \pv{64.2}\dci{\pv{0.46}} & \pv{86.1}\dci{\pv{1.18}} \\
GMT (causal) & \pv{72.9}\dci{\pv{0.06}} & \pv{62.6}\dci{\pv{0.22}} & \pv{77.8}\dci{\pv{0.45}} & \pv{5.9}\dci{\pv{0.12}} & \pv{16.3}\dci{\pv{0.56}} & \pv{67.0}\dci{\pv{0.58}} & \pv{86.2}\dci{\pv{0.28}} \\
\textbf{CoWeave} (ours) & \pv{80.5}\dci{\pv{0.50}} & \pv{69.3}\dci{\pv{0.27}} & \pv{86.5}\dci{\pv{0.48}} & \pv{2.5}\dci{\pv{0.10}} & \pv{11.0}\dci{\pv{0.54}} & \pv{82.1}\dci{\pv{0.45}} & \pv{94.9}\dci{\pv{0.31}} \\%
}
\def\StyPersistent{%
Independent & \pv{68.4} & \pv{65.5} & \pv{62.7} & \pv{58.4} & \pv{55.3} & \pv{80.9} \\
DyGLIP & \pv{70.3} & \pv{67.8} & \pv{65.3} & \pv{61.4} & \pv{58.6} & \pv{83.3} \\
ReST & \pv{72.7} & \pv{70.4} & \pv{68.2} & \pv{64.7} & \pv{62.2} & \pv{85.6} \\
MCTR & \pv{74.5} & \pv{72.2} & \pv{70.1} & \pv{66.7} & \pv{64.2} & \pv{86.1} \\
GMT (causal) & \tsecond{\pv{77.8}} & \tsecond{\pv{75.4}} & \tsecond{\pv{73.2}} & \tsecond{\pv{69.6}} & \tsecond{\pv{67.0}} & \tsecond{\pv{86.2}} \\
\rowcolor{tabours}\textbf{CoWeave} (ours) & \tbest{\pv{86.5}} & \tbest{\pv{85.5}} & \tbest{\pv{84.6}} & \tbest{\pv{83.1}} & \tbest{\pv{82.1}} & \tbest{\pv{94.9}} \\
$\Delta$ & \dgood{\pv{$+$8.7}} & \dgood{\pv{$+$10.1}} & \dgood{\pv{$+$11.4}} & \dgood{\pv{$+$13.5}} & \dgood{\pv{$+$15.1}} & \dgood{\pv{$+$8.7}} \\%
}
\def\StyStored{%
Independent & \pv{1.00} & \pv{1.00} & \pv{40.2}\dci{\pv{0.31}} & \pv{58.9}\dci{\pv{1.35}} & \pv{1.00} \\
DyGLIP & \pv{0.98} & \pv{1.00} & \pv{39.5}\dci{\pv{1.01}} & \pv{58.6}\dci{\pv{1.69}} & \pv{0.99} \\
ReST & \pv{0.93} & \pv{0.94} & \pv{37.5}\dci{\pv{0.62}} & \pv{55.5}\dci{\pv{0.57}} & \pv{0.88} \\
MCTR & \pv{1.24} & \pv{1.25} & \pv{49.8}\dci{\pv{1.01}} & \pv{73.4}\dci{\pv{1.11}} & \pv{0.71} \\
GMT (causal) & \pv{1.07} & \pv{1.08} & \pv{43.0}\dci{\pv{0.28}} & \pv{63.3}\dci{\pv{1.32}} & \pv{1.00} \\
\textbf{CoWeave} (ours) & \pv{1.16} & \pv{1.17} & \pv{46.6}\dci{\pv{1.04}} & \pv{68.7}\dci{\pv{2.45}} & \pv{0.94} \\%
}
\def\StyCost{%
Independent & \pv{28.73} & \pv{3.27} & \pv{32} & \pv{40.2} & \pv{68.8} \\
GMT (causal) & \pv{27.64} & \pv{4.36} & \pv{32} & \pv{43.0} & \tsecond{\pv{72.9}} \\
\rowcolor{tabours}\textbf{CoWeave} (ours) & \pv{24.82} & \pv{7.18} & \pv{32} & \pv{46.6} & \tbest{\pv{80.5}} \\%
}
\def\StyCrossed{%
Tracklet reader & GMT adapter & \pv{61.4} & \pv{72.1} & \pv{68.7} & \pv{66.3} & \pv{86.6} & \pv{45.2} & \pv{0.96} \\
Tracklet reader & CoWeave matcher & \tsecond{\pv{65.0}} & \pv{77.4} & \pv{75.2} & \tsecond{\pv{73.6}} & \tsecond{\pv{91.8}} & \pv{44.6} & \pv{0.96} \\
CoWeave reader & GMT adapter & \pv{64.6} & \tsecond{\pv{78.1}} & \tsecond{\pv{75.4}} & \pv{73.4} & \pv{89.9} & \pv{44.5} & \pv{0.96} \\
\rowcolor{tabours}CoWeave reader & CoWeave matcher & \tbest{\pv{69.3}} & \tbest{\pv{84.6}} & \tbest{\pv{83.1}} & \tbest{\pv{82.1}} & \tbest{\pv{94.9}} & \pv{46.6} & \pv{0.94} \\
$\Delta$ &  & \dgood{\pv{$+$7.9}} & \dgood{\pv{$+$12.5}} & \dgood{\pv{$+$14.4}} & \dgood{\pv{$+$15.8}} & \dgood{\pv{$+$8.3}} &  &  \\%
}
\def\StyBudget{%
0.25 & \pv{63.1} & \pv{65.1} & \tbest{\pv{74.2}} & \dgood{\pv{$+$9.1}} & \pv{71.4} \\
0.50 & \pv{66.5} & \pv{69.3} & \tbest{\pv{77.4}} & \dgood{\pv{$+$8.1}} & \pv{77.0} \\
1.00\,{\scriptsize\color{cwNote}default} & \pv{68.8} & \pv{72.9} & \tbest{\pv{80.5}} & \dgood{\pv{$+$7.6}} & \pv{82.1} \\
2.00 & \pv{70.0} & \pv{74.2} & \tbest{\pv{81.4}} & \dgood{\pv{$+$7.2}} & \pv{83.2} \\%
}
\def\StyValidity{%
0\%\,{\scriptsize\color{cwNote}default} & \pv{68.8} & \pv{72.9} & \tbest{\pv{80.5}} & \dgood{\pv{$+$7.6}} \\
10\% & \pv{68.8} & \pv{71.4} & \tbest{\pv{80.0}} & \dgood{\pv{$+$8.6}} \\
20\% & \pv{68.8} & \pv{69.4} & \tbest{\pv{79.4}} & \dgood{\pv{$+$10.0}} \\
30\% & \pv{68.8} & \pv{67.6} & \tbest{\pv{78.6}} & \dgood{\pv{$+$11.0}} \\
40\% & \pv{68.8} & \pv{65.8} & \tbest{\pv{77.6}} & \dgood{\pv{$+$11.8}} \\%
}
\def\StyDiagnostics{%
\rowcolor{tabgroup}\multicolumn{4}{l}{\textit{\textbf{Reliable relations and clear instance detail}}} \\
GMT (causal) & \pv{89.7} & \pv{3.2} & \pv{7.1} \\
\rowcolor{tabours}\textbf{CoWeave} (ours) & \tbest{\pv{95.6}} & \tbest{\pv{1.2}} & \tbest{\pv{3.2}} \\
$\Delta$ & \dgood{\pv{$+$5.9}} & \dgood{\pv{$-$2.0}} & \dgood{\pv{$-$3.9}} \\
\rowcolor{tabgroup}\multicolumn{4}{l}{\textit{\textbf{Shared group and weak instance detail}}} \\
GMT (causal) & \pv{65.4} & \pv{12.3} & \pv{22.3} \\
\rowcolor{tabours}\textbf{CoWeave} (ours) & \tbest{\pv{84.8}} & \tbest{\pv{3.3}} & \tbest{\pv{11.9}} \\
$\Delta$ & \dgood{\pv{$+$19.4}} & \dgood{\pv{$-$9.0}} & \dgood{\pv{$-$10.4}} \\
\rowcolor{tabgroup}\multicolumn{4}{l}{\textit{\textbf{Reappearance after group separation}}} \\
GMT (causal) & \pv{59.5} & \pv{15.4} & \pv{25.1} \\
\rowcolor{tabours}\textbf{CoWeave} (ours) & \tbest{\pv{84.1}} & \tbest{\pv{3.6}} & \tbest{\pv{12.3}} \\
$\Delta$ & \dgood{\pv{$+$24.6}} & \dgood{\pv{$-$11.8}} & \dgood{\pv{$-$12.8}} \\
\rowcolor{tabgroup}\multicolumn{4}{l}{\textit{\textbf{Invalid relations and valid instance evidence}}} \\
GMT (causal) & \pv{51.6} & \pv{21.3} & \pv{27.1} \\
\rowcolor{tabours}\textbf{CoWeave} (ours) & \tbest{\pv{83.2}} & \tbest{\pv{3.9}} & \tbest{\pv{12.9}} \\
$\Delta$ & \dgood{\pv{$+$31.6}} & \dgood{\pv{$-$17.4}} & \dgood{\pv{$-$14.2}} \\
\rowcolor{tabgroup}\multicolumn{4}{l}{\textit{\textbf{Complete symmetry (431 arrivals)}}} \\
GMT (causal) & \pv{0.0} & \pv{0.0} & \pv{100.0} \\
\rowcolor{tabours}\textbf{CoWeave} (ours) & \pv{0.0} & \pv{0.0} & \pv{100.0} \\
$\Delta$ & \dzero{\pv{0.0}} & \dzero{\pv{0.0}} & \dzero{\pv{0.0}} \\%
}
\def\StyAblation{%
\rowcolor{tabours}\textbf{Full CoWeave} & \tbest{\pv{80.5}} & \tbest{\pv{86.5}} & \tbest{\pv{2.5}} & \tbest{\pv{11.0}} & \tbest{\pv{82.1}} \\
Fixed retrieval & \tsecond{\pv{79.2}} & \tsecond{\pv{84.5}} & \tsecond{\pv{3.3}} & \tsecond{\pv{12.2}} & \tsecond{\pv{77.8}} \\
Zero relational support & \pv{77.1} & \pv{83.7} & \pv{3.5} & \pv{12.8} & \pv{77.0} \\
Fixed record ownership & \pv{76.5} & \pv{82.0} & \pv{3.8} & \pv{14.2} & \pv{74.9} \\
Without instance detail & \pv{74.4} & \pv{81.4} & \pv{4.5} & \pv{14.1} & \pv{73.4} \\%
}
\def\StyRetention{%
Recent & \pv{72.1} & \pv{74.2} & \pv{6.9} & \pv{18.9} & \pv{65.8} \\
Diverse & \tsecond{\pv{72.7}} & \pv{75.9} & \pv{6.5} & \tsecond{\pv{17.5}} & \pv{68.4} \\
Task-aware independent & \pv{72.1} & \tsecond{\pv{76.5}} & \tsecond{\pv{5.8}} & \pv{17.7} & \tsecond{\pv{70.4}} \\
\rowcolor{tabours}\textbf{CoWeave} (ours) & \tbest{\pv{80.5}} & \tbest{\pv{86.5}} & \tbest{\pv{2.5}} & \tbest{\pv{11.0}} & \tbest{\pv{82.1}} \\%
}
\def\StyIntervention{%
\rowcolor{tabours}\textbf{Original valid relations} & \tbest{\pv{69.3}} & \tbest{\pv{84.6}} & \tbest{\pv{83.1}} & \tbest{\pv{82.1}} & \tbest{\pv{94.9}} \\
No-operation control & \tbest{\pv{69.3}} & \tbest{\pv{84.6}} & \tbest{\pv{83.1}} & \tbest{\pv{82.1}} & \tbest{\pv{94.9}} \\
Degree-matched relation permutation & \tsecond{\pv{67.1}} & \tsecond{\pv{80.8}} & \tsecond{\pv{78.6}} & \tsecond{\pv{77.0}} & \tsecond{\pv{92.1}} \\
Zero relational support & \pv{66.1} & \tsecond{\pv{80.8}} & \tsecond{\pv{78.6}} & \tsecond{\pv{77.0}} & \pv{91.9} \\%
}
\def\StyCoverage{%
Independent & \pv{89.9} & \pv{83.8} & \pv{68.8} \\
GMT (causal) & \tsecond{\pv{92.0}} & \tsecond{\pv{86.9}} & \tsecond{\pv{72.9}} \\
\rowcolor{tabours}\textbf{CoWeave} (ours) & \tbest{\pv{96.9}} & \tbest{\pv{95.1}} & \tbest{\pv{80.5}} \\
$\Delta$ & \dgood{\pv{$+$4.9}} & \dgood{\pv{$+$8.2}} & \dgood{\pv{$+$7.6}} \\%
}
\def\StyRepair{%
\rowcolor{tabgroup}\multicolumn{5}{l}{\textit{\textbf{(a) 100 events that start from an erroneous ownership snapshot}}} \\
Frozen ownership & \tsecond{\pv{0}} & \tsecond{\pv{78}} & \tsecond{\pv{22}} & \tna \\
Frozen, no-operation replay & \tsecond{\pv{0}} & \tsecond{\pv{78}} & \tsecond{\pv{22}} & \tna \\
\rowcolor{tabours}\textbf{Revisable ownership} & \tbest{\pv{69}} & \tbest{\pv{15}} & \tbest{\pv{16}} & \tna \\
$\Delta$ & \dgood{\pv{$+$69}} & \dgood{\pv{$-$63}} & \dgood{\pv{$-$6}} &  \\
\rowcolor{tabgroup}\multicolumn{5}{l}{\textit{\textbf{(b) 200 events that start from correct ownership}}} \\
Frozen ownership & \tbest{\pv{190}} & \tbest{\pv{4}} & \pv{6} & \tbest{\pv{0}} \\
\rowcolor{tabours}\textbf{Revisable ownership} & \pv{188} & \pv{6} & \pv{6} & \pv{2} \\
$\Delta$ & \dbad{\pv{$-$2}} & \dbad{\pv{$+$2}} & \dzero{\pv{0}} & \dbad{\pv{$+$2}} \\%
}
\def\StyTraining{%
0 & \pv{0.6918}\dci{\pv{0.003}} & \pv{0.9977}\dci{\pv{0.003}} & \pv{69.1}\dci{\pv{0.07}} \\
25 & \pv{0.3833}\dci{\pv{0.001}} & \pv{0.6139}\dci{\pv{0.004}} & \pv{75.2}\dci{\pv{0.17}} \\
50 & \pv{0.2455}\dci{\pv{0.002}} & \pv{0.3581}\dci{\pv{0.003}} & \pv{78.5}\dci{\pv{0.06}} \\
75 & \pv{0.1853}\dci{\pv{0.003}} & \pv{0.2783}\dci{\pv{0.002}} & \pv{80.2}\dci{\pv{0.17}} \\
100 & \pv{0.1681}\dci{\pv{0.002}} & \pv{0.2481}\dci{\pv{0.003}} & \pv{80.7}\dci{\pv{0.13}} \\%
}
\def\StyBootstrap{%
\rowcolor{tabgroup}\multicolumn{4}{l}{\textit{\textbf{CoWeave $-$ GMT (causal) on MTMMC}}} \\
G-IDF1 & \dgood{\pv{$+$7.57}} & \pv{[$+$6.57, $+$8.68]} & $\checkmark$ \\
Correct & \dgood{\pv{$+$8.67}} & \pv{[$+$7.19, $+$10.15]} & $\checkmark$ \\
Wrong & \dgood{\pv{$-$3.41}} & \pv{[$-$3.73, $-$3.09]} & $\checkmark$ \\
$P_{30}$ & \dgood{\pv{$+$15.04}} & \pv{[$+$13.23, $+$16.77]} & $\checkmark$ \\
\rowcolor{tabgroup}\multicolumn{4}{l}{\textit{\textbf{CoWeave $-$ GMT (causal) on other datasets}}} \\
WILDTRACK G-IDF1 & \dgood{\pv{$+$4.60}} & \pv{[$+$3.46, $+$5.74]} & $\checkmark$ \\
MMPTrack G-IDF1 & \dgood{\pv{$+$7.40}} & \pv{[$+$6.90, $+$7.90]} & $\checkmark$ \\
DIVOTrack G-IDF1 & \dgood{\pv{$+$6.20}} & \pv{[$+$4.71, $+$7.69]} & $\checkmark$ \\
\rowcolor{tabgroup}\multicolumn{4}{l}{\textit{\textbf{Reader $\times$ matcher interaction on MTMMC}}} \\
G-IDF1 & \pv{$+$0.88} & \pv{[$-$1.21, $+$2.89]} & \textcolor{cwNote}{no} \\
$P_{30}$ & \pv{$+$1.34} & \pv{[$-$1.62, $+$4.20]} & \textcolor{cwNote}{no} \\%
}
\def\StyReference{%
\rowcolor{tabgroup}\multicolumn{3}{l}{\textit{\textbf{Same causal RGB stream}}} \\
GMT (causal) & {\color{cwNote}Same RGB observations} & \pv{72.9} \\
\rowcolor{tabours}\textbf{CoWeave} (ours) & {\color{cwNote}Same RGB observations} & \tbest{\pv{80.5}} \\
\rowcolor{tabgroup}\multicolumn{3}{l}{\textit{\textbf{Additional information}}} \\
OCMCTrack & {\color{cwNote}Additional geometry} & \pv{76.0} \\
Lifted multicut & {\color{cwNote}Future tracklets} & \tsecond{\pv{78.7}} \\%
}
\def\StyTransfer{%
\rowcolor{tabgroup}\multicolumn{9}{l}{\textit{\textbf{WILDTRACK}}} \\
Independent & \pv{65.0} & \pv{54.9} & \pv{64.8} & \pv{9.6} & \pv{25.6} & \pv{50.7} & \pv{78.3} & \pv{40.8} \\
DyGLIP & \pv{67.9} & \pv{56.6} & \pv{65.5} & \pv{8.8} & \pv{25.8} & \pv{54.3} & \pv{82.9} & \pv{39.3} \\
ReST & \pv{68.4} & \pv{58.2} & \pv{68.8} & \pv{8.1} & \pv{23.1} & \pv{59.1} & \tsecond{\pv{85.9}} & \pv{37.8} \\
MCTR & \pv{69.1} & \pv{59.7} & \pv{70.9} & \pv{7.2} & \pv{21.9} & \pv{58.9} & \pv{83.1} & \pv{50.2} \\
GMT (causal) & \tsecond{\pv{70.2}} & \tsecond{\pv{60.3}} & \tsecond{\pv{74.6}} & \tsecond{\pv{7.0}} & \tsecond{\pv{18.4}} & \tsecond{\pv{63.5}} & \pv{85.1} & \pv{42.8} \\
\rowcolor{tabours}\textbf{CoWeave} (ours) & \tbest{\pv{74.8}} & \tbest{\pv{65.2}} & \tbest{\pv{80.2}} & \tbest{\pv{3.4}} & \tbest{\pv{16.4}} & \tbest{\pv{73.2}} & \tbest{\pv{91.2}} & \pv{47.1} \\
$\Delta$ & \dgood{\pv{$+$4.6}} & \dgood{\pv{$+$4.9}} & \dgood{\pv{$+$5.6}} & \dgood{\pv{$-$3.6}} & \dgood{\pv{$-$2.0}} & \dgood{\pv{$+$9.7}} & \dgood{\pv{$+$6.1}} &  \\
\rowcolor{tabgroup}\multicolumn{9}{l}{\textit{\textbf{MMPTrack}}} \\
Independent & \pv{61.9} & \pv{52.2} & \pv{61.1} & \pv{9.9} & \pv{28.9} & \pv{47.7} & \pv{78.1} & \pv{39.6} \\
DyGLIP & \pv{63.9} & \pv{54.4} & \pv{63.8} & \pv{9.3} & \pv{26.9} & \pv{51.6} & \pv{80.9} & \pv{39.2} \\
ReST & \pv{65.8} & \pv{55.6} & \pv{64.6} & \pv{8.5} & \pv{26.9} & \pv{55.4} & \tsecond{\pv{85.9}} & \pv{37.6} \\
MCTR & \pv{66.1} & \pv{57.5} & \pv{68.1} & \pv{7.7} & \pv{24.2} & \pv{56.2} & \pv{82.5} & \pv{49.1} \\
GMT (causal) & \tsecond{\pv{66.6}} & \tsecond{\pv{57.6}} & \tsecond{\pv{70.7}} & \tsecond{\pv{7.3}} & \tsecond{\pv{22.0}} & \tsecond{\pv{59.9}} & \pv{84.7} & \pv{42.7} \\
\rowcolor{tabours}\textbf{CoWeave} (ours) & \tbest{\pv{74.0}} & \tbest{\pv{64.4}} & \tbest{\pv{81.0}} & \tbest{\pv{3.1}} & \tbest{\pv{15.9}} & \tbest{\pv{75.5}} & \tbest{\pv{93.2}} & \pv{46.2} \\
$\Delta$ & \dgood{\pv{$+$7.4}} & \dgood{\pv{$+$6.8}} & \dgood{\pv{$+$10.3}} & \dgood{\pv{$-$4.2}} & \dgood{\pv{$-$6.1}} & \dgood{\pv{$+$15.6}} & \dgood{\pv{$+$8.5}} &  \\
\rowcolor{tabgroup}\multicolumn{9}{l}{\textit{\textbf{DIVOTrack}}} \\
Independent & \pv{58.5} & \pv{50.2} & \pv{58.2} & \pv{10.8} & \pv{31.0} & \pv{44.6} & \pv{76.7} & \pv{40.7} \\
DyGLIP & \pv{61.0} & \pv{51.4} & \pv{59.8} & \pv{9.8} & \pv{30.4} & \pv{47.2} & \pv{79.0} & \pv{39.4} \\
ReST & \pv{61.8} & \pv{52.9} & \pv{62.0} & \pv{9.2} & \pv{28.8} & \pv{51.6} & \pv{83.2} & \pv{38.1} \\
MCTR & \pv{62.6} & \tsecond{\pv{55.6}} & \pv{63.3} & \pv{8.4} & \pv{28.3} & \pv{54.6} & \tsecond{\pv{86.3}} & \pv{50.6} \\
GMT (causal) & \tsecond{\pv{63.1}} & \pv{54.6} & \tsecond{\pv{67.4}} & \tsecond{\pv{7.8}} & \tsecond{\pv{24.8}} & \tsecond{\pv{56.0}} & \pv{83.1} & \pv{42.5} \\
\rowcolor{tabours}\textbf{CoWeave} (ours) & \tbest{\pv{69.3}} & \tbest{\pv{60.8}} & \tbest{\pv{74.0}} & \tbest{\pv{4.0}} & \tbest{\pv{22.0}} & \tbest{\pv{68.3}} & \tbest{\pv{92.3}} & \pv{46.4} \\
$\Delta$ & \dgood{\pv{$+$6.2}} & \dgood{\pv{$+$6.2}} & \dgood{\pv{$+$6.6}} & \dgood{\pv{$-$3.8}} & \dgood{\pv{$-$2.8}} & \dgood{\pv{$+$12.3}} & \dgood{\pv{$+$9.2}} &  \\%
}
\def\StySweeps{%
$\lambda_U$ & \pv{0.1}: \pv{79.1}\,/\,\pv{80.3} & \pv{0.2}: \pv{80.3}\,/\,\pv{81.8} & \cellcolor{tabours}\pv{0.35}: \pv{80.5}\,/\,\pv{82.1} & \pv{0.5}: \pv{80.3}\,/\,\pv{81.8} & \pv{0.7}: \pv{79.9}\,/\,\pv{81.3} \\
$\lambda_B$ & \pv{0.1}: \pv{78.3}\,/\,\pv{79.3} & \pv{0.25}: \pv{80.1}\,/\,\pv{81.6} & \cellcolor{tabours}\pv{0.5}: \pv{80.5}\,/\,\pv{82.1} & \pv{1}: \pv{80.0}\,/\,\pv{81.4} & \pv{2}: \pv{78.6}\,/\,\pv{79.6} \\
$\lambda_{\mathrm{rel}}$ & \pv{0.1}: \pv{77.0}\,/\,\pv{77.0} & \pv{0.25}: \pv{79.3}\,/\,\pv{80.4} & \pv{0.5}: \pv{80.2}\,/\,\pv{81.7} & \cellcolor{tabours}\pv{1}: \pv{80.5}\,/\,\pv{82.1} & \pv{2}: \pv{80.1}\,/\,\pv{81.5} \\
Temperature $T$ & \pv{0.25}: \pv{79.0}\,/\,\pv{80.2} & \pv{0.5}: \pv{80.2}\,/\,\pv{81.7} & \cellcolor{tabours}\pv{1}: \pv{80.5}\,/\,\pv{82.1} & \pv{1.5}: \pv{80.3}\,/\,\pv{81.8} & \pv{2}: \pv{79.9}\,/\,\pv{81.4} \\
Candidate limit & \pv{8}: \pv{77.6}\,/\,\pv{77.7} & \pv{16}: \pv{79.6}\,/\,\pv{80.7} & \cellcolor{tabours}\pv{32}: \pv{80.5}\,/\,\pv{82.1} & \pv{48}: \pv{80.3}\,/\,\pv{81.8} & \pv{64}: \pv{79.9}\,/\,\pv{81.3} \\
Hypothesis beam & \pv{4}: \pv{77.8}\,/\,\pv{78.6} & \pv{8}: \pv{79.6}\,/\,\pv{81.0} & \cellcolor{tabours}\pv{16}: \pv{80.5}\,/\,\pv{82.1} & \pv{24}: \pv{80.3}\,/\,\pv{81.9} & \pv{32}: \pv{80.0}\,/\,\pv{81.5} \\
Decision beam & \pv{2}: \pv{78.3}\,/\,\pv{78.9} & \pv{4}: \pv{79.8}\,/\,\pv{81.0} & \cellcolor{tabours}\pv{8}: \pv{80.5}\,/\,\pv{82.1} & \pv{12}: \pv{80.4}\,/\,\pv{81.9} & \pv{16}: \pv{80.1}\,/\,\pv{81.5} \\%
}
