# Supplementary material for: CoWeave: Identity-Specific Context Reasoning for Persistent Multi-Camera Tracking
Source: arXiv:2611.38993 source file (2026-11-28)
Supplement: Supplementary file 6 [file supp_preamble.tex]

\usepackage{graphicx,amsmath,amssymb,booktabs,xspace,multirow}
\setlength{\parskip}{0pt}
\AtBeginDocument{\flushbottom}
\makeatletter
\def\cvprsection{\@startsection{section}{1}{\z@}{-10pt}{.001pt}{\large\bf}}
\def\cvprsubsection{\@startsection{subsection}{2}{\z@}{-11.98pt}{.001pt}{\elvbf}}
\newcommand{\cwdisplayskips}{\abovedisplayskip=.5\baselineskip\belowdisplayskip=.5\baselineskip
  \abovedisplayshortskip=.5\baselineskip\belowdisplayshortskip=.5\baselineskip}
\g@addto@macro\normalsize{\cwdisplayskips}
\AtBeginDocument{\cwdisplayskips}
\newcommand{\gridfix}[1]{\abovedisplayskip=\dimexpr.5\baselineskip+(#1)/2\relax
  \belowdisplayskip=\abovedisplayskip\abovedisplayshortskip=\abovedisplayskip\belowdisplayshortskip=\abovedisplayskip}
\setlength{\floatsep}{14pt}\setlength{\textfloatsep}{14pt}\setlength{\intextsep}{14pt}
\setlength{\dblfloatsep}{14pt}\setlength{\dbltextfloatsep}{14pt}
\newsavebox{\cw@fbox}\newdimen\cw@fh
\newenvironment{gridfloat}[1][0]{\def\cw@extra{#1}\begin{lrbox}{\cw@fbox}\begin{minipage}[b]{\linewidth}}{\end{minipage}\end{lrbox}%
  \cw@fh=\dimexpr\ht\cw@fbox+\dp\cw@fbox+\textfloatsep\relax
  \@tempcnta=\numexpr\cw@fh/\baselineskip+\cw@extra\relax
  \usebox{\cw@fbox}\par\vspace{\dimexpr\@tempcnta\baselineskip-\cw@fh\relax}}
\makeatother
\newcommand{\runin}[1]{\par\noindent\textbf{#1}\hspace{0.5em}\ignorespaces}
\AtBeginDocument{\captionsetup[table]{skip=5pt}}

\usepackage{array,tabularx,colortbl}
\definecolor{tabours}{HTML}{E3EEF9}\definecolor{tabgroup}{HTML}{EFF1F3}
\definecolor{tabgood}{HTML}{2E8B3E}\definecolor{tabbad}{HTML}{C0392B}\definecolor{tabci}{HTML}{8C8C8C}
\newcommand{\tbest}[1]{\textbf{#1}}
\newcommand{\tsecond}[1]{\underline{#1}}
\newcommand{\dgood}[1]{\textcolor{tabgood}{#1}}
\newcommand{\dbad}[1]{\textcolor{tabbad}{#1}}
\newcommand{\tna}{\textcolor{tabci}{--}}
\newcommand{\dzero}[1]{\textcolor{tabci}{#1}}
\newcolumntype{C}{>{\centering\arraybackslash}X}
\newcommand{\dci}[1]{{\color{tabci}\scriptsize$\,\pm$#1}}
\usepackage{tikz}\usetikzlibrary{arrows.meta,positioning,calc,shadows.blur,fadings}
\usepackage{pgfplots}\pgfplotsset{compat=1.18}\usepgfplotslibrary{fillbetween}
\usepackage{anyfontsize}
\DeclareMathSizes{7}{7}{6}{6}% figure text: sub/superscripts stay >= 6pt in print
\DeclareMathSizes{8}{8}{6}{6}
\input{figures/tikz/supp_coweave_style}
\ifdefined\pdfminorversion\pdfminorversion=7\fi
\newcommand{\method}{CoWeave\xspace}
\definecolor{pvyellow}{rgb}{1,0.93,0.2}
\newcommand{\pv}[1]{#1}% numbers confirmed by the authors on 2026-11-14; the macro is kept so generated tables need no change
\usepackage{soul}
\sethlcolor{pvyellow}
\soulregister{\cite}{7}\soulregister{\ref}{7}\soulregister{\emph}{1}
\newcommand{\pvs}[1]{\hl{#1}}
\DeclareMathOperator*{\argmax}{arg\,max}
\DeclareMathOperator*{\argmin}{arg\,min}
\newcommand{\R}{\mathbb{R}}
\newcommand{\E}{\mathbb{E}}
\newcommand{\ind}{\mathbf{1}}
